# Supplementary material for: Exploring Factors and Metrics to Select Open Source Software Components for Integration: An Empirical Study
Source: arXiv:2102.09977 source file (2022-02-04)
Supplement: Supplementary file 2 [file AppendixABackup.tex]

\begin{enumerate}
    \item \textbf{Personal Information}
    \begin{enumerate}
        \item Name
        \item Age
        \item Role
        \item Time in the company (years)
        \item Unit/Department
    \end{enumerate}
    \item \textbf{General Questions regarding OSS Adoption}
    \begin{enumerate}
        \item How experienced are you with OSS?
        \item Are you following any specific model for selecting OSS or are you adapting any model to your needs? If yes, which changes are you applying to the standard model?
        \item What are the key factors that you consider when you adopt OSS? How important is each factor from 0 to 5?, where 0 means not important at all, and 5 means extremely important?
        \item What factors do you think personally important? How important is each factor from 0 to 5, where 0 means not important at all, and 5 means extremely important?
        \begin{enumerate}[label*=\arabic*.]
            \item [F1:] Community \& Support
            \item Documentation
            \item License
            \item Operational SW Characteristics
            \item Maturity
            \item Quality
            \item Trustworthiness
            \item Risk
        \end{enumerate}
    \end{enumerate}
    \item \textbf{Community and Support}
    \begin{enumerate}
        \item Community Attributes
        \begin{enumerate}[label*=\arabic*.]
            \item What are the most important community attributes that you consider when adopting OSS? How important is each factor from 0 to 5, where 0 means not important at all, and 5 means extremely important?
            \begin{enumerate}[label*=\arabic*.]
                \item Community Reputation
                \item Community Size
            \end{enumerate}
            \item How about community reputation? Any factors? How important is each factor from 0 to 5, where 0 means not important at all, and 5 means extremely important?
            \item How do you measure community size? How important is each metric from 0 to 5, where 0 means not important at all, and 5 means extremely important?
            \begin{enumerate}[label*=\arabic*.]
                \item Number of contributors
                \item Number of subscribers
                \item Community age
                \item Number of involved developers per company
                \item Number of independent developers
            \end{enumerate}
        \end{enumerate}
        \item Community Support \\
        How important is community support? (0 = not important at all, 5 = extremely important)
        \begin{enumerate}[label*=\arabic*.]
            \item How do you measure community support? Any factors? How important is each factor from 0 to 5, where 0 means not important at all, and 5 means extremely important?
            \begin{enumerate}[label*=\arabic*.]
                \item Communication
                \item Involvement
                \item Sustainability
            \end{enumerate}
            \item How do you measure communication? Any factors? How important is each factor from 0 to 5, where 0 means not important at all, and 5 means extremely important?
            \begin{enumerate}[label*=\arabic*.]
                \item Availability of questions/answers
                \item Availability of forum
                \item Number of mailing list
                \item Traffic on the mailing list
                \item Responsiveness of postings
                \item Friendliness
                \item Relation between stakeholders
                \item Quality of postings
            \end{enumerate}
            \item How do you measure involvement? Any factors? How important is each factor from 0 to 5, where 0 means not important at all, and 5 means extremely important?
            \begin{enumerate}[label*=\arabic*.]
                \item Coordination
                \item Clear project management
            \end{enumerate}
            \item How do you measure sustainability? Any factors? How important is each factor from 0 to 5, where 0 means not important at all, and 5 means extremely important?
            \begin{enumerate}[label*=\arabic*.]
                \item Existence of maintainer
                \item Maturity implications of Mailing List Support
            \end{enumerate}
        \end{enumerate}
        \item Popularity
        \begin{enumerate}[label*=\arabic*.]
            \item How do you measure community popularity? Any factors? How important is each factor from 0 to 5, where 0 means not important at all, and 5 means extremely important?
            \begin{enumerate}[label*=\arabic*.]
                \item Number of downloads
                \item Number of watches
                \item Number of stars
                \item Number of forks
            \end{enumerate}
        \end{enumerate}
    \end{enumerate}
    \item \textbf{Documentation}
    \begin{enumerate}
        \item What are the key factors of documentation you consider when you adopt OSS? How important is each factor from 0 to 5, where 0 means not important at all, and 5 means extremely important?
        \begin{enumerate}[label*=\arabic*.]
            \item Documentation completeness
            \item Availability of documentation/books/online docs
            \item Availability of development process documentation
            \item Reference documentation
            \item Tutorial/guidelines documentation
            \item Quality report
            \item Usage documentation
            \item Best practices
            \item Availability of architectural documentation 
            \item Distribution media
            \item Software requirements
            \item Hardware requirements
            \item Test case documentation
            \item Coding comments
        \end{enumerate}
        \item Test Case Documentation
        \begin{enumerate}[label*=\arabic*.]
            \item How do you measure test case documentation? Any factors? How important is each factor from 0 to 5, where 0 means not important at all, and 5 means extremely important?
            \begin{enumerate}[label*=\arabic*.]
                \item Trace links between code and test cases
                \item Trace links between issues and code
            \end{enumerate}
        \end{enumerate}
    \end{enumerate}
    \item \textbf{License}
    \begin{enumerate}
        \item How do you measure license? Any factors? How important is each factor from 0 to 5, where 0 means not important at all, and 5 means extremely important?
        \begin{enumerate}[label*=\arabic*.]
            \item License type
            \item Law conformance
        \end{enumerate}
    \end{enumerate}
    \item \textbf{Operational Software Characteristics}
    \begin{enumerate}
        \item How do you measure operational software characteristics? Any factors? How important is each factor from 0 to 5, where 0 means not important at all, and 5 means extremely important?
        \begin{enumerate}[label*=\arabic*.]
            \item Trialability
            \item Independence from other SW
            \item Development language
            \item Programming language uniformity
            \item Multiplatform support
            \item Standard compliance
        \end{enumerate}
    \end{enumerate}
    \item \textbf{Maturity}
    \begin{enumerate}
        \item How do you measure maturity? Any factors? How important is each factor from 0 to 5, where 0 means not important at all, and 5 means extremely important?
        \begin{enumerate}[label*=\arabic*.]
            \item Number of forks
            \item Stability
            \item Number of releases
            \item Number of releases per period
            \item Age
            \item Number of commits
            \item Number of bug reports
            \item Development versions
            \item System growth
        \end{enumerate}
    \end{enumerate}
    \item \textbf{Quality}
    \begin{enumerate}
        \item How do you measure quality? Any factors? How important is each factor from 0 to 5, where 0 means not important at all, and 5 means extremely important?
        \begin{enumerate}[label*=\arabic*.]
            \item Resilience
            \item Reliability
            \item Performances
            \item Security
            \item Modularity
            \item Usability
            \item Portability
            \item Flexibility/Exploitability
            \item Code quality
            \item Coding practices
            \item Mainteinability
            \item Update/Upgrade/Add-ons/Plugin
            \item Visibility
            \item Development process
            \item As-is utility/Quality in use/ External quality
            \item Efficiency
            \item Architecture
        \end{enumerate}
        \item Reliability
        \begin{enumerate}[label*=\arabic*.]
            \item How do you measure reliability? Any factors? How important is each factor from 0 to 5, where 0 means not important at all, and 5 means extremely important?
            \begin{enumerate}[label*=\arabic*.]
                \item Component reliability
                \item Architecture reliability
                \item System reliability
                \item Number of faults(open, closed, ...)/Fault density
                \item Average fault age
                \item Mean time between software failure (MTBF)
            \end{enumerate}
        \end{enumerate}
        \item Performance
        \begin{enumerate}[label*=\arabic*.]
            \item How do you measure performance? Any factors? How important is each factor from 0 to 5, where 0 means not important at all, and 5 means extremely important?
        \end{enumerate}
        \item Security
        \begin{enumerate}[label*=\arabic*.]
            \item How do you measure security? Any factors? How important is each factor from 0 to 5, where 0 means not important at all, and 5 means extremely important?
            \begin{enumerate}[label*=\arabic*.]
                \item Number security vulnerability code
                \item Information for security
            \end{enumerate}
        \end{enumerate}
        \item Modularity
        \begin{enumerate}[label*=\arabic*.]
            \item How do you measure modularity? Any factors? How important is each factor from 0 to 5, where 0 means not important at all, and 5 means extremely important?
        \end{enumerate}
        \item Usability
        \begin{enumerate}[label*=\arabic*.]
            \item How do you measure usability? Any factors? How important is each factor from 0 to 5, where 0 means not important at all, and 5 means extremely important?
            \begin{enumerate}[label*=\arabic*.]
                \item Understandability
                \item Operability
                \item Learnability
            \end{enumerate}
        \end{enumerate}
        \item Portability
        \begin{enumerate}[label*=\arabic*.]
            \item How do you measure portability? Any factors? How important is each factor from 0 to 5, where 0 means not important at all, and 5 means extremely important?
            \begin{enumerate}[label*=\arabic*.]
                \item Adaptability 
                \item Installability
            \end{enumerate}
        \end{enumerate}
        \item Flexibility/Exploitability
        \begin{enumerate}[label*=\arabic*.]
            \item How do you measure flexibility/exploitability? Any factors? How important is each factor from 0 to 5, where 0 means not important at all, and 5 means extremely important?
        \end{enumerate}
        \item Code Quality
        \begin{enumerate}[label*=\arabic*.]
            \item How do you measure code quality? Any factors? How important is each factor from 0 to 5, where 0 means not important at all, and 5 means extremely important?
            \begin{enumerate}[label*=\arabic*.]
                \item Code complexity (class, methods, ...)
                \item Change proneness
                \item Fault proneness
                \item Test coverage
                \item Longevity
                \item Code size
                \item Technical difficulty
                \item Coding conventions
            \end{enumerate}
            \item How do you measure longevity? Any factors? How important is each factor from 0 to 5, where 0 means not important at all, and 5 means extremely important?
            \begin{enumerate}[label*=\arabic*.]
                \item Age of product
                \item Version numbers
            \end{enumerate}
            \item How do you measure conventions? Any factors? How important is each factor from 0 to 5, where 0 means not important at all, and 5 means extremely important?
            \begin{enumerate}[label*=\arabic*.]
                \item Method calling conventions
                \item Class naming conventions
                \item Loop/Switch/If conventions
                \item Public/Private conventions
                \item Overriding conventions
            \end{enumerate}
        \end{enumerate}
        \item Code Practices
        \begin{enumerate}[label*=\arabic*.]
            \item How do you measure code practices? Any factors? How important is each factor from 0 to 5, where 0 means not important at all, and 5 means extremely important?
            \begin{enumerate}[label*=\arabic*.]
                \item Usage of Linters,
                \item Definition of customs/rules for Linters
                \item Issue/Commit traceability
            \end{enumerate}
        \end{enumerate}
        \item Product Team
        \begin{enumerate}[label*=\arabic*.]
            \item How do you measure project team? Any factors? How important is each factor from 0 to 5, where 0 means not important at all, and 5 means extremely important?
            \begin{enumerate}[label*=\arabic*.]
                \item Developer quality
                \item Productivity
            \end{enumerate}
        \end{enumerate}
        \item Mainteinability
        \begin{enumerate}[label*=\arabic*.]
            \item How do you measure mainteinability? Any factors? How important is each factor from 0 to 5, where 0 means not important at all, and 5 means extremely important?
            \begin{enumerate}[label*=\arabic*.]
                \item Analyzability
                \item Testability
                \item Changeability
                \item Availability and type of Defect management system
                \item Availability and type of Version management system
                \item Opened defects
                \item Source code changes/modificability
                \item Resolved defects
                \item Fixed defects
                \item Enhancements
                \item Resolving time for non-fixed defects
                \item Resolving time for fixed defects
                \item Resolved defects life cycle
                \item Fixed defects life cycles
                \item Detect initiated source code changes
                \item Defect proneness
            \end{enumerate}
        \end{enumerate}
        \item Update/Upgrade/Add-ons/Plugin
        \begin{enumerate}[label*=\arabic*.]
            \item How do you measure update/upgrade/add-ons/plugin? Any factors? How important is each factor from 0 to 5, where 0 means not important at all, and 5 means extremely important?
        \end{enumerate}
        \item Visibility
        \begin{enumerate}[label*=\arabic*.]
            \item How do you measure visibility? Any factors? How important is each factor from 0 to 5, where 0 means not important at all, and 5 means extremely important?
        \end{enumerate}
        \item Development process
        \begin{enumerate}[label*=\arabic*.]
            \item How do you measure development process? Any factors? How important is each factor from 0 to 5, where 0 means not important at all, and 5 means extremely important?
        \end{enumerate}
        \item As-is utility/Quality in use/External quality?
        \begin{enumerate}[label*=\arabic*.]
            \item How do you measure as-is utility/quality in use/external quality? Any factors? How important is each factor from 0 to 5, where 0 means not important at all, and 5 means extremely important?
            \begin{enumerate}[label*=\arabic*.]
                \item Effectiveness
                \item Efficiency
                \item Satisfaction
                \item Freedom from risk
                \item Context coverage
            \end{enumerate}
            \item How do you measure satisfaction? Any factors? How important is each factor from 0 to 5, where 0 means not important at all, and 5 means extremely important?
            \begin{enumerate}[label*=\arabic*.]
                \item Usefulness
                \item Trust
                \item Pleasure
                \item Comfort
            \end{enumerate}
            \item How do you measure freedom from risk? Any factors? How important is each factor from 0 to 5, where 0 means not important at all, and 5 means extremely important?
            \begin{enumerate}[label*=\arabic*.]
                \item Economic risk migration
                \item Health \& safety risk migration
                \item Environmental risk migration
            \end{enumerate}
        \end{enumerate}
        \item Efficiency
        \begin{enumerate}[label*=\arabic*.]
            \item How do you measure efficiency? Any factors? How important is each factor from 0 to 5, where 0 means not important at all, and 5 means extremely important?
        \end{enumerate}
        \item Architecture
        \begin{enumerate}[label*=\arabic*.]
            \item How do you measure architecture? Any factors? How important is each factor from 0 to 5, where 0 means not important at all, and 5 means extremely important?
        \end{enumerate}
    \end{enumerate}
    \item \textbf{Risk}
    \begin{enumerate}
        \item How do you measure risks? Any factors? How important is each factor from 0 to 5, where 0 means not important at all, and 5 means extremely important?
        \begin{enumerate}[label*=\arabic*.]
            \item Perceived lack of confidentiality
            \item Perceived lack of integrity
            \item Perceived high availability
            \item Perceived high structural assurance
            \item Business risks
        \end{enumerate}
        \item How do you measure business risk? Any factors? How important is each factor from 0 to 5, where 0 means not important at all, and 5 means extremely important?
        \begin{enumerate}[label*=\arabic*.]
            \item Strategic risks
            \item Operational risks
            \item Financial risks
            \item Hazard risks
        \end{enumerate}
    \end{enumerate}
    \item \textbf{Trustworthiness}
    \begin{enumerate}
        \item How do you measure trustworthiness? Any factors? How important is each factor from 0 to 5, where 0 means not important at all, and 5 means extremely important?
        \begin{enumerate}[label*=\arabic*.]
            \item Component trustworthiness
            \item Architecture trustworthiness
            \item System trustworthiness
            \item Functional requirements satisfaction
            \item Customer satisfaction/requirements
            \item Interoperability
            \item Facilities for modifying and customizing
            \item OSS provider reputation
            \item Interface language localization
            \item Existence of benchmark/test
            \item Collaboration with other product
        \end{enumerate}
        \item How do you measure collaboration with other product? Any factors? How important is each factor from 0 to 5, where 0 means not important at all, and 5 means extremely important?
        \begin{enumerate}[label*=\arabic*.]
            \item Commercial vendor integrations
            \item Community-created integrations 
            \item The percentage of existing needed integrations
        \end{enumerate}
    \end{enumerate}
    \item \textbf{Others}
    \begin{enumerate}
        \item Are there other factors left?
        \begin{enumerate}[label*=\arabic*.]
            \item Staffing
            \item Technical environment
            \item Assessment results from 3rd parties
            \item Voluntariness of use
            \item Results demonstrability
            \item Configuration management
            \item Personal interest
            \item Regulation and political influence
            \item Accomplishment
            \item Ethical reasons
            \item Experience stimulation
        \end{enumerate}
    \end{enumerate}
\end{enumerate}
